# Supplementary material for: Modeling bias in decision-making attractor networks
Source: arXiv:2508.07471 source file (2025-08-10)
Supplement: Supplementary file 3 [file ListOfSymbols.tex]

% Place the list of symbols below.
\begin{eqlist}[\labelsep 1em]

\item[$\alpha$]
The first greek letter, p.~\pageref{ChX-figure: FigureLabel3}

\item[$\alpha$]
The first greek letter, p.~\pageref{ChX-figure: FigureLabel3}

\item[$\alpha$]
The first greek letter, but we should really add some more text, though we need it to go on two lines, p.~\pageref{ChX-figure: FigureLabel7}

\item[$\alpha$]
The first greek letter, p.~\pageref{ChX-figure: FigureLabel3}

\item[$\alpha$]
The first greek letter, p.~\pageref{ChX-figure: FigureLabel4}

\item[$\alpha$]
The first greek letter, p.~\pageref{ChX-figure: FigureLabel5}

\item[$\alpha$]
The first greek letter, p.~\pageref{ChX-figure: FigureLabel6}

\item[$\alpha$]
The first greek letter, p.~\pageref{ChX-figure: FigureLabel7}

\item[$\alpha$]
The first greek letter, p.~\pageref{ChX-figure: FigureLabel8}

\item[$\alpha$]
The first greek letter, p.~\pageref{ChX-figure: FigureLabel9}

\item[$\alpha$]
The first greek letter, p.~\pageref{ChX-figure: FigureLabel10}

\item[$\alpha$]
The first greek letter, p.~\pageref{ChX-figure: FigureLabel3}

\item[$\alpha$]
The first greek letter, p.~\pageref{ChX-figure: FigureLabel4}

\item[$\alpha$]
The first greek letter, p.~\pageref{ChX-figure: FigureLabel5}

\item[$\alpha$]
The first greek letter, p.~\pageref{ChX-figure: FigureLabel6}

\item[$\alpha$]
The first greek letter, p.~\pageref{ChX-figure: FigureLabel7}

\item[$\alpha$]
The first greek letter, p.~\pageref{ChX-figure: FigureLabel8}

\item[$\alpha$]
The first greek letter, p.~\pageref{ChX-figure: FigureLabel3}

\item[$\alpha$]
The first greek letter, p.~\pageref{ChX-figure: FigureLabel3}

\item[$\alpha$]
The first greek letter, p.~\pageref{ChX-figure: FigureLabel3}

\item[$\alpha$]
The first greek letter, p.~\pageref{ChX-figure: FigureLabel3}

\item[$\alpha$]
The first greek letter, p.~\pageref{ChX-figure: FigureLabel3}

\item[$\alpha$]
The first greek letter, p.~\pageref{ChX-figure: FigureLabel3}

\item[$\alpha$]
The first greek letter, p.~\pageref{ChX-figure: FigureLabel3}

\end{eqlist}
